# Supplementary material for: SpotServe: Serving Generative Large Language Models on Preemptible Instances
Source: arXiv:2311.15566 source file (2023-11-27)
Supplement: Supplementary file 1 [file appendix.tex]

\section{Device Mapping for Multi-GPU Instances}
\begin{algorithm}[ht]
\small
\begin{algorithmic}[1]

\Function{DeviceMapper}{$\m{V}_a, \m{V}_t, \m{E}$}
    \State $\hat{G} \gets \min(G, M)$
    \State $\hat{\m{V}}_a, \hat{\m{V}}_t, \hat{\m{E}} \gets$ \texttt{NodeFusion}$(\m{V}_a, \m{V}_t, \m{E}, \hat{G})$
    \For{each fused edge $\hat{e}_{\hat{u}\hat{v}}\in \hat{\m{E}}$}
    \State $\m{E}_{\hat{u}\hat{v}}$ $\gets$ \texttt{KM-Mactch}$(\hat{u}, \hat{v}, \m{E})$
    \State $\hat{e}_{\hat{u}\hat{v}}$.\texttt{weight}$\gets \max\{e.$\texttt{weight}$\mid e\in \m{E}_{\hat{u}\hat{v}}\}$ 
    % \State $\hat{e}_{\hat{u}\hat{v}}$.\texttt{weight} $\gets$ \texttt{KM-Mactch}$(\hat{u}, \hat{v}, \m{E})$
    \EndFor
    \State $\hat{\m{E}}_{\hat{\m{V}}_a\hat{\m{V}}_t}\gets$\texttt{KM-Match}$(\hat{\m{V}}_a, \hat{\m{V}}_t, \hat{\m{E}})$
\EndFunction
\end{algorithmic}
\caption{Two-step device mapping algorithm.}
\label{algo:map}
\end{algorithm}

Since each GPU instance may consist of multiple GPUs (i.e., $G\geq 1$) with higher inter-GPU bandwidth, we facilitate the hierarchical architecture by fusing these adjacent GPUs, and the pipeline-stage-shard position in the same tensor model parallel group is fused as well. 
% \CA{Algorithm will match inside all possible fused node pairs at first, and do a final match on the fused nodes, where weights are given by the first-step matching}. 
As shown in Algorithm~\ref{algo:map}, we prioritize to perform the KM match within each fused group and generate the new weight of the fused edge. Then we do another round of KM match on the fused graph.

\section{Full 12-hour trace}
\begin{figure}[ht]
    \centering
    \includegraphics[width=\linewidth]{figures/g4dn_trace.pdf}
    \caption{The trace segments we chose from real g4dn trace.}
    \label{g4dn_trace}
\end{figure}

\section{Case Study on Fixed Arrival Rate}
\begin{figure}[h]
    \centering
    \includegraphics[width=\linewidth]{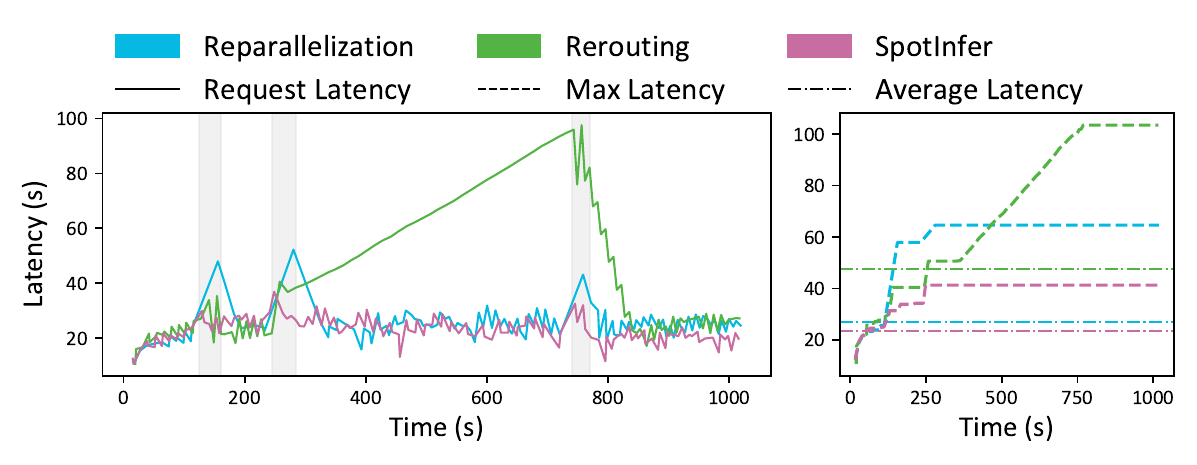}
    \caption{Case study of request latency for GPT-20B model on trace $B_S$, as well as the average and accumulated max latency.}
    \label{fig:case_study_0506}
\end{figure}

To provide a better understanding of the superior performance of \Sys, we also conduct an additional case study on trace $B_S$ with GPT-20B model (0.35 requests/s), since it's more comprehensible. The left part of Figure~\ref{fig:case_study_0506} illustrates the per-request latency during the entire trace, and the right part shows the corresponding average latency and the accumulated max latency (i.e., the maximum latency from the beginning till now). Based on trace $B_S$, there are ten instances at the beginning but two of them are preempted at $t=120s$ and another one gets preempted at $t=240s$. The rest seven instances continue the inference process for 480s until two new instances become available at $t=720s$ and $t=960s$ individually.

At the beginning, \Sys and all baselines start idle instances. At $t=120s$, two instances are lost and one of them comes from the utilized instance, so we have to handle this preemption to maintain the configuration of (2,2,8) using the rest eight instances. Reparallelization simply terminates and restarts all inference processes, resulting in a high peak request latency. Rerouting only terminates a single inference pipeline and restarts another one, leading to a relatively lower tail latency compared with Reparallelization. \Sys proactively migrates the model and cache contexts to the alive idle instance and achieves the lowest tail latency.

At $t=240s$, there are only seven instances left and the original configuration degrades to (1,2,8). But Reparallelization and \Sys can obtain a new parallel configuration (2,3,4) and perform the configuration adjustment for lower latency in the future.
The new instances has to recover the model context from S3 which can be 9.54$\times$ slower than the context migration in \Sys. While the alive instances can load the model from the local disk which also needs extra 45\% recovery overhead even with a warm-up.
As shown in the left part of Figure~\ref{fig:case_study_0506}, Rerouting starts to accumulate requests from 240s since the throughput is too low to handle arriving requests, while Reparallelization and \Sys can almost maintain a stable request latency with (2,3,4), which has much higher throughput with slightly higher inference latency.

At $t=720s$, the new coming instance turns the configuration back to (2,2,8) for all approaches while \Sys has the lowest peak latency again.

\section{Robustness to Arrival Rate}
\begin{figure}[ht]
    \centering
    \includegraphics[width=\linewidth]{figures/tpt.pdf}
    \caption{End-to-end GPT-20B serving performance with different arrival rates.}
    \label{fig:tpt}
\end{figure}

We also study the system's robustness to the arrival rate of input requests on GPT-20B model. 
Besides the original fixed arrival rate of 0.35 requests/s, we add two more arrival rates of 0.25 requests/s and 0.55 requests/s to see the difference. 
The P99 tail latency and the average latency are shown in Figure~\ref{fig:tpt} for both traces. 
We can find that as the arrival rate increases, all three approaches have a higher inference latency than before. 
For trace $B_S$, the increasing of the arrival rate leads to overload for Rerouting and incurs significantly high latency. 
Another finding is that adding on-demand instances in time can avoid overload for Rerouting but it is still facing higher latency compared with \Sys.
Due to higher peak latency when migration, which need much more time to serve stacked requests under a high arrival rate.
As a result, \Sys has a more significant advantage over Rerouting and Reparallelization in terms of average latency on Trace $B_{S+O}$: \Sys gains the average latency speedup from $1.54\times$ to $1.92\times$ over Rerouting and from $1.19\times$ to $1.47\times$ over Reparallelization under arrival rate 0.55.

When arrival rate is low (i.e. 0.25), the parallization controller of \Sys will return the totally same configuration as Rerouting. In this case, the performance of Rerouting is quite close to \Sys. As we mentioned in \S\ref{sec:eval}, its KV-cache maintenance and faster recovery speed are beneficial to lower migration overhead. \Sys slightly outweighs Rerouting and both of them obviously outperform Reparallelization due to lower migration overhead.

% \CA{The Greater arrival rates, the higher end-to-end latency. For A0.25, Triton's configuration is totally the same as \Sys, our incremental is discussed above (\Sys v.s. Triton : migration)}

% Moreover, we use two more arrival rates 0.25 and 0.55 for OPT 20B to study the effect of different arrival rates on same model.

Figure \ref{fig:tpt} shows the performance of the three serving systems under different arrival rates on GPT 20B with Trace $B_S$ and Trace $B_{S+O}$. When arrival rate is higher (i.e. 0.55), the overload on Rerouting is much more severe than that under arrival rate 0.35, the P99 latency speedup of \Sys comparing to Rerouting increases from $2.67\times$ to $3.46\times$. Meanwhile, although Trace $B_{S+O}$ does not meet overload, both Rerouting and Reparallelization need take much more time to counteract the end-to-end latency peak caused by migration. What is worse is that higher migration overhead than \Sys result in more requests stacking during the migration. As a result, \Sys has a better advantage over Rerouting and Reparallelization in terms of average latency on Trace $B_{S+O}$: \Sys gains the average latency speedup from $1.54\times$ to $1.92\times$ over Rerouting and from $1.19\times$ to $1.47\times$ over Reparallelization under arrival rate 0.55.

When arrival rate is lower (i.e. 0.25), configuration (1,2,8) will not cause overload, and parallelization controller of \Sys will return the totally same configuration as Rerouting. At this time, the performance of Rerouting is quite close to \Sys. \Sys's KV-cache maintenance and faster recovery speed are beneficial to lower migration overhead, thus \Sys slightly outweighs Rerouting and both of them obviously outperform Reparallelization due to lower migration overhead.

% \CA{Anything more to add? I have no idea.}

% \section{More Case Study Results}

% \begin{figure}[ht]
%     \centering
%     \includegraphics[width=\linewidth]{figures/ablation_study_0304.pdf}
%     \caption{Ablation study for GPT-20B on trace $A_S$.}
%     \label{fig:ablation_0304}
% \end{figure}
% \begin{figure}[ht]
%     \centering
%     \includegraphics[width=\linewidth]{figures/ablation_study_0506.pdf}
%     \caption{Ablation study for GPT-20B on trace $B_S$.}
%     \label{fig:ablation_0506}
% \end{figure}
